# Supplementary material for: The StatCan Dialogue Dataset: Retrieving Data Tables through Conversations with Genuine Intents
Source: arXiv:2304.01412 source file (2023-04-05)
Supplement: Supplementary file 1 [file DialogueAnalysis.pdf]

# Analysis

We include the conversation ID based on the order index in the dataset. The speech acts are written in blue, followed by a semi-colon, at the end of each message. This analysis is done for 100 turns of user-operator interactions, following the data categories specifications.

## Conversation 1365

**Turns: 2**

**Messages: 6**

<user>: hi, i was wondering if you vae any statistics on video game sales, ot high school drop out rates? infoSeekingQuestions; request;

<operator>: Hello my name is Sylvain, how may I help you? offer;

<user>: hello, I am looking for high school drop out r ates and teen depression rates, but cant seem to find anything that goes back more than a year request;

<operator>: Data for High School dropouts is compiled by the Provincial Education Ministry. To obtain this infor please contact the Education Ministry of your province inform; promise;

<operator>: Data for mood disorder (depression) is available on our website from the Data Table 13- 10-0096-18 (https://www150.statcan.gc.ca/t1/tbl1/en/tv.action?pid=1310009618) answer;

<operator>: To view/ manipulate the variables available in a data table: • Click on "Add/Remove data" • Select at least one variable in each tab and click on “Apply” in order to view your customized table To download the data: • Click on “Download” • Select one of the three output formats then click on the hyperlink and save the table The following video may also be helpful to you: How to use the data tables (https://www.statcan.gc.ca/eng/sc/video/howto) . inform; request;

## Conversation 20341

**Turns: 3**

**Messages: 11**

<user>: Hello, I am looking for a list of current populations of each city and town in Manitoba for CancerCare Manitoba. is this something that I can find here? request; infoSeekingQuestions;

<operator>: Hello, my name is Jimmy N., how may I help you? offer;

<operator>: What do you mean for CancerCare Manitoba? clarificationQuestion;

<user>: I work at a health centre called CancerCare Manitoba answer;

<operator>: Oh ok. Please hold while I find the information. autoFeedback; timeManagement;

<operator>: You can obtain this information at the following hyperlink : Population and dwelling counts, for Canada, provinces and territories, census metropolitan areas and census agglomerations, 2016 and 2011 censuses â€“ 100% data (https://www12.statcan.gc.ca/census-recensement/2016/dp-pd/hlt-fst/pd-pl/Table.cfm?Lang=Eng&T=201&SR=1&S=3&O=D&RPP=25) answer;

<user>: Is there any current information from either 2018 or 2019? clarificationQuestion;

<operator>: Please hold while I find the information. timeManagement; promise;

<operator>: You can have an estimate of the population at the following hyperlink : Table: 17-10-0135-01 Population estimates, July 1, by census metropolitan area and census agglomeration, 2016 boundaries (https://www150.statcan.gc.ca/t1/tbl1/en/cv.action?pid=1710013501) answer;

<operator>: To view/ manipulate the variables available in a data table: â€¢ Click on "Add/Remove data" â€¢ Click on the â€œ + â€  icon next to a checkbox to expand the list of variables (if applicable) â€¢ Select at least one variable in each tab and click on â€œApplyâ€ in order to view your customized table To download the data: â€¢ Click on â€œDownloadâ€ â€¢ Select one of the three output formats then click on the hyperlink and save the table The following video may also be helpful to you:  How to use the data tables (https://www.statcan.gc.ca/eng/sc/video/howto) . inform; instruct;

<operator>: Dear customer, this chat was closed automatically due to inactivity. inform;

## Conversation 8500

**Turns: 3**

**Messages: 9**

<user>: Hi. I want to know how many small, medium and big companies are there in canada. Thank you request;

<operator>: Hello, my name is Olivier C. Please wait while i find the information you're looking for. timeManagement; promise;

<operator>: Thank you for waiting, you will find the information about the number of business per business size if you click the following hyperlinks : Canadian Business Counts, with employees, December 2019 (https://www150.statcan.gc.ca/t1/tbl1/en/tv.action?pid=3310022201) Canadian Business Counts, without employees, December 2019 (https://www150.statcan.gc.ca/t1/tbl1/en/tv.action?pid=3310022301) answer;

<operator>: To view/ manipulate the variables available in a data table: • Click on "Add/Remove data" • Click on the “ + ” icon next to a checkbox to expand the list of variables (if applicable) • Select at least one variable in each tab and click on “Apply” in order to view your customized table To download the data: • Click on “Download” • Select one of the three output formats then click on the hyperlink and save the table The following video may also be helpful to you: How to use the data tables (https://www.statcan.gc.ca/eng/sc/video/howto) . inform; instruct;

<user>: But what about data about companies with employees ? clarificationQuestion;

<operator>: it's the first link i gave you : Canadian Business Counts, with employees, December 2019 (https://www150.statcan.gc.ca/t1/tbl1/en/tv.action?pid=3310022201) inform; answer

<operator>: You have to modify the table to obtain detailled information per number of employees. instruct;

<user>: Ok! Thank you very much ! autoFeedback;

<operator>: You're welcome.

## Conversation 22204

**Turns: 4**

**Messages: 12**

<user>: hi, i just wonder why when I hit the apply and it just start endless loading? infoSeekingQuestions;

<user>: screenshot.lzsc (https://www.statcan.gc.ca/livechat/getfile.php?file=screenshot.lzsc&id=f68501a42839a8fc4bad6b96b9776020)

<operator>: Hello, my name is Jeremie. Which table are you on? Can you provide me with the hyperlink or the table number so I can better assist you? infoSeekingQuestions;

<user>: https://www150.statcan.gc.ca/t1/tbl1/en/cv.action?pid=1310045101#archived

<operator>: Ok, so you selected a combination of variables in the "Customize table" feature and it could not load properly? infoSeekingQuestions; autoFeedback;

<user>: yes autoFeedback; answer;

<user>: I basely just change the period and the indicator inform;

<operator>: Ok, I've tried manipulating the table myself and it seems to work fine. Depending on the number of variables you added, it might take longer for the table to load, but normally the updated table should appear just fine below. autoFeedback; inform;

<user>: ok, thanks i will try again autoFeedback;

<user>: have a good day

<operator>: You are welcome, if the problem persists, send us an email at infostats@canada.ca (mailto:infostats@canada.ca) and provide the variables you need, we might be able to either fix the table or send you the data you need in an Excel file. offer;

<operator>: Dear customer, this chat was closed automatically due to inactivity. inform;

## Conversation 17928

**Turns: 4**

**Turns: 10**

<user>: What data set would you recommend using to for analysis of job specific post secondary education employment rates? infoSeekingQuestions;

<operator>: Hello, my name is Martine, let me check.. promise; timeManagement;

<user>: okay. Thank you autoFeedback;

<operator>: Occupation - National Occupational Classification (NOC) 2016 (693A), Highest Certificate, Diploma or Degree (15), Labour Force Status (3), Age (13A) and Sex (3) for the Labour Force Aged 15 Years and Over in Private Households of Canada, Provinces and Territories, Census Metropolitan Areas and Census Agglomerations, 2016 Census - 25% Sample Data (https://www12.statcan.gc.ca/census-recensement/2016/dp-pd/dt-td/Rp-eng.cfm?LANG=E&APATH=3&DETAIL=0&DIM=0&FL=A&FREE=0&GC=0&GID=0&GK=0&GRP=1&PID=110696&PRID=10&PTYPE=109445&S=0&SHOWALL=0&SUB=0&Temporal=2017&THEME=124&VID=0&VNAMEE=&VNAMEF=) answer;

<operator>: Labour force characteristics by educational degree, monthly, unadjusted for seasonality (https://www150.statcan.gc.ca/t1/tbl1/en/tv.action?pid=1410011701) answer;

<user>: Is there a data set that incorporates all the information included in both of these? infoSeekingQuestions;

<operator>: There is not. That would be a custom product. To order these, contact us at 1-800-263-1136 answer; offer;

<user>: Thank you Martine

<operator>: You are welcome.

<operator>: Dear customer, this chat was closed automatically due to inactivity. inform;

# Conversation 3555

**Turns: 4**

**Messages: 12**

<user>: Hello - I'm wondering if it is possible to find out how many people in the country/in each province are getting paid a certain hourly wage using public statcan data. Specifically, I am looking for: request;

<user>: - the number of people that make $15/hour

<user>: - the number of people that make between $15-$20/hour

<operator>: Hello, please wait while I try to find this information for you. timeManagement;

<user>: Okay thank you autoFeedback;

<operator>: I'm sorry for the wait. After looking for the wages information we have, they all seem to be related to average wage by either industry or occupation. For example, look at the following table: Employee wages by occupation, annual (https://www150.statcan.gc.ca/t1/tbl1/en/tv.action?pid=1410034001) answer;

<operator>: The only table that I was able to find that has backets is the following: Upper income limit, income share and average of adjusted market, total and after-tax income by income decile (https://www150.statcan.gc.ca/t1/tbl1/en/tv.action?pid=1110019301) ,then again the table does not have the wages variable you are looking for. inform;

<operator>: The information you are looking for might be available as a custom order

<user>: No problem about the wait - thank you for looking!

<user>: I will take a look at those tables and consider making a custom order if I end up still needing more information inform;

<operator>: To obtain a free cost estimate for this service, please send us your request, clearly indicating the variables, geographic areas, time frame and data frequency needed, making sure to include your complete contact information (name of organization, address, postal code, and phone number) at the following email address: infostats@canada.ca (mailto:infostats@canada.ca) or by telephone at 1-800-263- 1136. Our agents are available Monday to Friday (except holidays) from 7:30 am to 7:30 pm (Eastern Time). An agent will get in touch with you to verify the information, provide an estimate and proceed with the payment, if applicable. Please do not share any personal information through the live chat. 10/9/2019 2/2 Once you send your request, please provide the following case #: 941065. inform;

<user>: Okay thank you for that information, much appreciated

# Conversation 4890

**Turns: 8**

**Messages: 21**

<user>: Thank you for your information, but I have done that already. Your previous website had a "manipulate" function to calculate the percentage change. I don't see the button anymore, and wondered if you have other schedule prepared as that function is gone. inform; request;

<operator>: Hello, my name is Jimmy N., how may I help you? offer;

<user>: I was talking with Sylvain, will you be able to see the log? inform; infoSeekingQuestions;

<operator>: Yes, please hold while I verify. promise; autoFeedback; timeManagement;

<operator>: Just to clarify, you're looking for all-items ? clarificationQuestion;

<user>: Ideally, I want the percentage change for these items: https://www150.statcan.gc.ca/t1/tbl1/en/tv.action?pid=1810000401 request;

<operator>: You can obtain this information at the following hyperlink : Table: 18-10- 0004-13 Consumer Price Index by product group, monthly, percentage change, not seasonally adjusted, Canada, provinces, Whitehorse, Yellowknife and Iqaluit (https://www150.statcan.gc.ca/t1/tbl1/en/tv.action?pid=1810000413) answer;

<operator>: To view/ manipulate the variables (like the reference period) available in a data table: • Click on "Add/Remove data" • Click on the “ + ” icon next to a checkbox to expand the list of variables (if applicable) • Select at least one variable in each tab and click on “Apply” in order to view your customized table To download the data: • Click on “Download” • Select one of the three output formats then click on the hyperlink and save the table The following video may also be helpful to you: How to use the data tables (https://www.statcan.gc.ca/eng/sc/video/howto) . inform; instruct;

<operator>: You also have the following interactive tool : Consumer Price Index Data Visualization Tool (https://www150.statcan.gc.ca/n1/pub/71-607-x/2018016/cpilg-ipcgl-eng.htm) inform;

<user>: I hope you are not a machine... I got the exact same answer previously, which did not answer my question. I CANNOT pick multiple reference periods in this sheet. Like I requested 11/13/2019 2/2 before, I would like to get the continuous percentage change from Jan 2000 up to now. How can I get that data? infoSeekingQuestions; inform; request;

<operator>: All the CPI data tables are showing a monthly percentage change depending on the month of reference. inform;

<operator>: Did you take a look at interactive tool? clarificationQuestion;

<user>: OHHHHHHHHH! autoFeedback;

<user>: THANK YOU SO MUCH!

<operator>: You're welcome!

<user>: I was trying the first one you mentioned. inform;

<operator>: We are currently evaluating our customer service. Your input would be much appreciated: www.statcan.gc.ca/survey/SIS (http://www.statcan.gc.ca/survey/SIS) Thank you! inform;

<user>: Yes, this is exactly I needed. autoFeedback; inform;

<operator>: I'm glad that helped ! Have a great day!

<user>: You too.

<operator>: Thank you!

## Conversation 18839

**Turns: 3**

**Messages: 8**

<user>: Hi team, can you please help me retrieve data of public deposits of chartered banks? infoSeekingQuestions; request;

<operator>: Please hold timeManagement;

<user>: Surely. autoFeedback;

<operator>: You can obtain this info on our website from our Data Table 10-10-0116-01 (https://www150.statcan.gc.ca/t1/tbl1/en/tv.action?pid=1010011601) answer;

<operator>: To view/ manipulate the variables available in a data table: â€¢ Click on "Add/Remove data" â€¢ Select at least one variable in each tab and click on â€œApplyâ€  in order to view your customized table To download the data: â€¢ Click on â€œDownloadâ€  â€¢ Select one of the three output formats then click on the hyperlink and save the table The following video may also be helpful to you:Â How to use the data tables (https://www.statcan.gc.ca/eng/sc/video/howto) . inform; instruct;

<operator>: Please take note that this is a non-Statistics Canada Table. This info is provide from The Bank of Canada inform;

<user>: Thanks a lot! So, how should I get down to Public deposits? or rather which of these lines would direct me to Public deposits? clarificationQuestion;

<operator>: Under the category Chartered bank deposits. For more info please contact The Bank of Canada on their website by using their Online Request Form (https://www.bankofcanada.ca/about/contact-information/general-inquiries/#online) answer; inform;

## Conversation 11600

**Turns: 4**

**Messages: 18**

<user>: hello

<user>: how are you?

<operator>: Hello, my name is Jimmy N.

<operator>: I'm good, thank you for asking. How may I help you? offer;

<user>: Hi Jimmy

<user>: I am looking for a table similar which has data similar to this infographic link request;

<user>: https://www150.statcan.gc.ca/n1/pub/11-627-m/11-627-m2018053-eng.htm

<user>: expenditures by household type

<operator>: You can obtain that information at the following hyperlink : Table: 11-10-0224-01 - Household spending by household type (https://www150.statcan.gc.ca/t1/tbl1/en/cv.action?pid=1110022401) answer;

<operator>: To view/ manipulate the variables available in a data table: • Click on "Add/Remove data" • Click on the “ + ” icon next to a checkbox to expand the list of variables (if applicable) • Select at least one variable in each tab and click on “Apply” in order to view your customized table To download the data: • Click on “Download” • Select one of the six output formats then click on the hyperlink and save the table The following video may also be helpful to you: How to use the data tables (https://www.statcan.gc.ca/eng/sc/video/howto) . inform; instruct;

<user>: oh that's great! autoFeedback;

<user>: Thanks a lot!

<operator>: You're welcome!

<operator>: Do you have any other questions? infoSeekingQuestions;

<user>: No thanks! You gave me what I was searching found request;

<user>: :)

<user>: have a good day

<operator>: Thank you for contacting Statistics Canada. Have a great day as well !

# Conversation 24047

**Turns: 4**

**Messages: 9**

<user>: how do i change data to percentage through your website infoSeekingQuestions;

<operator>: Please wait while I try to find this information for you. timeManagement; promise;

<operator>: some tables will display data as percentages, others will not automatically. If that is the case, you can always calculate the percentages yourself. What percentage are you looking for? answer; clarificationQuestion;

<user>: unemployment rate in canada 2007 - 2017 (ages 15-24) answer;

<operator>: ok, please hold while I look this up autoFeedback; timeManagement; promise;

<user>: ok autoFeedback;

<operator>: Labour force characteristics by industry, annual (https://www150.statcan.gc.ca/t1/tbl1/en/cv!recreate.action?pid=1410002301&selectedNodeIds=2D6,5D2&checkedLevels=0D1,2D1,2D2,2D3,2D4,3D1&refPeriods=20070101,20170101&dimensionLayouts=layout2,layout2,layout3,layout2,layout2,layout2&vectorDisplay=false) answer;

<operator>: To view/ manipulate the variables available in a data table: â€¢ Click on "Add/Remove data" â€¢ Click on the â€œ + â€  icon next to a checkbox to expand the list of variables (if applicable) â€¢ Select at least one variable in each tab and click on â€œApplyâ€ in order to view your customized table To download the data: â€¢ Click on â€œDownloadâ€ â€¢ Select one of the three output formats then click on the hyperlink and save the table The following video may also be helpful to you:Â How to use the data tables (https://www.statcan.gc.ca/eng/sc/video/howto) . inform; instruct;

<user>: thanks graham i appreciate it

# Conversation 4174

**Turns: 5**

**Messages: 16**

<user>: Can you give the total number of births in Canada for 1990, 1991, 1992, 1993 and 1994? I don't want a chart I want the total number please request; infoSeekingQuestions; inform;

<operator>: Hello, my name is Jimmy. Please hold while I find the information. timeManagement; promise;

<operator>: I have data up to 1991.

<operator>: 1991=402,533 1992= 398,643 1993=388,394 1994=385,114 inform;

<user>: Great thanks very much. Can you also give me the numbers for 2000, 2001, 2002, 2003, 2004, 2005 as well autoFeedback; request;

<operator>: You're welcome, please hold while I find the information. timeManagement; promise;

<operator>: 2000=327,882 2001=333,744 2002=328,802 2003=335,202 2004=337,072 2005=342,176 answer;

<user>: Thanks so much can I ask for one more date. 2008 and 2009 request;

<operator>: Sure, please hold. timeManagement; promise;

<operator>: 2008=377,886 and 2009=380,863 answer;

<user>: Can I ask one more question -- are these numbers on a calendar basis -- January to December??? clarificationQuestion;

<operator>: Yes it's the total from January to December for each of those year. answer;

<operator>: If you wish to obtain more information, please visit the following hyperlink : Table: 13-10-0415-01 Live births, by month (https://www150.statcan.gc.ca/t1/tbl1/en/cv.action?pid=1310041501) inform;

<operator>: To view/ manipulate the variables available in a data table: • Click on "Add/Remove data" • Click on the “ + ” icon next to a checkbox to expand the list of variables (if applicable) • Select at least one variable in each tab and click on “Apply” in order to view your customized table To download the data: • Click on “Download” • Select one of the three output formats then click on the hyperlink and save the table The following video may also be helpful to you: How to use the data tables 10/23/2019 2/2 (https://www.statcan.gc.ca/eng/sc/video/howto) . inform; instruct;

<user>: Thanks so much, you have been a great help! Have a good day!

<operator>: You're welcome. Thank you and have a nice day as well!

# Conversation 28

**Turns: 2**

**Messages: 11**

<user>: Hi there - My name's Sebastian. I'm trying to find a StatCan table

<user>: related to annual Grain production in Ontario with Farm Gate Value request;

<operator>: Hello, my name is Amy, thank you for contacting Statistics Canada.

<operator>: Thank you. Please wait while I try to find this information for you. timeManagement; promise;

<user>: Thanks Amy!

<user>: Table: 32-10-0015-01 seems to come close; though it only seems to have select months? inform;

<operator>: You will find here a data table containing statistics on Grain production by province https://www150.statcan.gc.ca/t1/tbl1/en/tv.action?pid=3210035101 (https://www150.statcan.gc.ca/t1/tbl1/en/tv.action?pid=3210035101) answer;

<operator>: Additionnally, this one gives detailed data on crop, but only at the Canada level, not for just Ontario : https://www150.statcan.gc.ca/t1/tbl1/en/tv.action?pid=3210035901 (https://www150.statcan.gc.ca/t1/tbl1/en/tv.action?pid=3210035901) answer;

<operator>: Regarding the one you found (Farm supply and disposition of grains, 32-10-0015-01) you can view additional months by doing the following : inform;

<operator>: Click on "Add/Remove reference period" Select the months and years you'd like to see Click on “Apply” in order to view your customized table instruct;

<operator>: Dear customer, this chat was closed automatically due to inactivity. Inform;

# Conversation 7198

**Turns: 4**

**Messages: 20**

<user>: Hello. I would like to know if this is the latest data on Canadian childhood obesity request;

<user>: Measured children and youth body mass index (BMI) (World Health Organization classification), by age group and sex, Canada and provinces, Canadian Community Health Survey - Nutrition1 2 3 4

<user>: measured in 2015

<operator>: Please hold timeManagement;

<operator>: Self reported obesity is available for people age group 12 to 17 13-10-0096-21 (https://www150.statcan.gc.ca/t1/tbl1/en/tv.action?pid=1310009621) answer;

<user>: but measured is this? clarificationQuestion;

<operator>: For age 5 to 79 13-10-0373-01 (https://www150.statcan.gc.ca/t1/tbl1/en/tv.action?pid=https://www150.statcan.gc.ca/t1/tbl1/en/tv.action? pid=1310037301) answer;

<user>: this last one did not work inform;

<user>: 13-10-0795-01

<user>: is this the last one? clarificationQuestion;

<operator>: 13-10-0373-01 (https://www150.statcan.gc.ca/t1/tbl1/en/tv.action?pid=1310037301) answer;

<operator>: view/ manipulate the variables available in a data table: • Click on "Add/Remove data" • Click on the “ + ” icon next to a checkbox to expand the list of variables (if applicable) • Select at least one variable in each tab and click on “Apply” in order to view your customized table To download the data: • Click on “Download” • Select one of the three output formats then click on the hyperlink and save the table The following video may also be helpful to you: How to use the data tables (https://www.statcan.gc.ca/eng/sc/video/howto) .  inform; instruct;

<user>: thanks 03/02/2020 2/2

<user>: so the latest measured is from 2017, is that correct? clarificationQuestion;

<operator>: You're welcome

<operator>: Correct answer;

<user>: perfect1 autoFeedback;

<user>: thank you very much

<user>: have a good day!

<operator>: You're welcome

## Conversation 8750

**Turns: 2**

**Messages: 5**

<user>: Hi, I am looking for statistics for Ottawa income according to age group request;

<operator>: Hello, please wait while I try to find this information for you. timeManagement; promise;

<user>: ok. thanks autoFeedback;

<operator>: Thank you for your patience. I was able to find the following table: Distribution of total income by census family type and age of older partner, parent or individual (https://www150.statcan.gc.ca/t1/tbl1/en/cv.action?pid=1110001201) To view/ manipulate the variables available in a data table: • Click on "Add/Remove data" • Click on the “ + ” icon next to a checkbox to expand the list of variables (if applicable) • Select at least one variable in each tab and click on “Apply” in order to view your customized table To download the data: • Click on “Download” • Select one of the three output formats then click on the hyperlink and save the table The following video may also be helpful to you: How to use the data tables (https://www.statcan.gc.ca/eng/sc/video/howto) . inform; instruct; answer;

<operator>: Dear customer, this chat was closed automatically due to inactivity.

# Conversation 23136

**Turns: 3**

**Messages: 6**

<user>: Hi where can i find the list of top 5 most populated cities in canada infoSeekingQuestions;

<operator>: Hello, my name is Jeremie. Let me search our most recent population estimates for you. timeManagement; promise;

<user>: ok autoFeedback;

<operator>: We don't have a table that gives, in order, the "top 5" most populated cities in Canada, but this table gives the most recent estimates of 2018 for all the major cities in Canada : Table 17-10-0135-01 Population estimates, July 1, by census metropolitan area and census agglomeration, 2016 boundaries (https://www150.statcan.gc.ca/t1/tbl1/en/tv.action?pid=1710013501) answer;

<user>: ok thanks autoFeedback;

<operator>: You are welcome! If you have the time, we are currently evaluating our customer service. Your input would be much appreciated:Â www.statcan.gc.ca/survey/SIS (http://www.statcan.gc.ca/survey/SIS) Â Thank you! inform; request;

## Conversation 8960

**Turns: 6**

**Messages: 17**

<user>: This is pretty cool!

<operator>: Hello, my name is Martine, how may I help you? offer;

<user>: I have a question - how would I be able to access data for 2019 on the amount of money the federal government spent (money out) to Canadians through social programs like EI / OAS etc... infoSeekingQuestions;

<operator>: Letme check. timeManagement;

<user>: Thank you

<operator>: Revenue, expenditure and budgetary balance - General governments (x 1,000,000) (https://www150.statcan.gc.ca/t1/tbl1/en/tv.action?pid=3610047701) answer;

<user>: This is in billions correct? clarificationQuestion;

<operator>: No you mutiply by 1 million as indicated in the title. answer;

<user>: Okay thank you......this is amazing thank you so much

<user>: But please stay as I digest timeManagement;

<user>: So where would I be looking for social programs like OAS? clarificationQuestion;

<user>: And can this be filtered for Ontario?

<operator>: No this is for Canada inform;

<operator>: Revenue, expenditure and budgetary balance - General governments, provincial and territorial economic accounts (x 1,000,000) (https://www150.statcan.gc.ca/t1/tbl1/en/tv.action?pid=3610045001) answer;

<user>: So if I were to assume correctly that "Contributions to social insurance plans" would include things like OAS and EI? infoSeekingQuestions;

<operator>: Yes answer;

<operator>: Dear customer, this chat was closed automatically due to inactivity. Inform;

## Conversation 19161

**Turns: 4**

**Messages: 12**

<user>: Hi, i would like to find yearly GDP growth of Canada please request;

<user>: and well as yearly unemployment rate since 2010

<operator>: Hello, my name is Jimmy. Please hold while I find the information. timeManagement; promise;

<user>: thank you Jimmy

<operator>: You can obtain this information by clicking the following hyperlinks :Gross domestic product, expenditure-based, provincial and territorial, annual (x 1,000,000)Gross domestic product (GDP) at basic prices, by industry (x 1,000,000) (https://www150.statcan.gc.ca/t1/tbl1/en/tv.action?pid=3610022201) Labour force characteristics by industry, annual (x 1,000) (https://www150.statcan.gc.ca/t1/tbl1/en/tv.action?pid=1410032702) answer;

<operator>: To view/ manipulate the variables available in a data table: â€¢ Click on "Add/Remove data" â€¢ Select at least one variable in each tab and click on â€œApplyâ€  in order to view your customized table To download the data: â€¢ Click on â€œDownloadâ€  â€¢ Select one of the three output formats then click on the hyperlink and save the table The following video may also be helpful to you:Â How to use the data tables (https://www.statcan.gc.ca/eng/sc/video/howto) . inform; instruct;

<operator>: Do you have any other question? offer;

<user>: is there a place where i could find the yearly growth on GDP? without the calculation? infoSeekingQuestions;

<user>: like for example i am getting 1.7% GDP growth in 2017 from a source but i believe it was higher, i was wondering if you have the percentage number handy inform;

<operator>: You can obtain this information at the following hyperlink : Gross domestic product (GDP) at basic prices, by industry, provinces and territories, growth rates (x 1,000,000) (https://www150.statcan.gc.ca/t1/tbl1/en/tv.action?pid=3610040202) answer;

<user>: thank you

<operator>: You're welcome!

# Conversation 4196

**Turns: 4**

**Messages: 10**

<user>: Hi, I was wondering if you have any health data on the Tk'emlups Te Secwepemc band? infoSeekingQuestions;

<operator>: Hello, my name is Olivier C. Please wait while i'm searching for this information. timeManagement; promise;

<user>: okay! autoFeedback;

<operator>: Thank you for wiating. Unfortunately, the only health indicators that we have is based on the aboriginal identity : First nation, metis, inuit answer;

<user>: Oh I see, can you point me in the direction of First Nations health indicators? request;

<operator>: Of course, simply click on the following hyperlinks to access information about health indicators by aboriginal identity : Health indicator estimates (https://www150.statcan.gc.ca/t1/tbl1/en/tv.action?pid=1310009901) . Perceived general health by Aboriginal identity (https://www150.statcan.gc.ca/t1/tbl1/en/tv Aboriginal identity (https://www150.statcan.gc.ca/t1/tbl1/en/tv.action?pid=4110000301) . Perceived mental health and suicidal thoughts by Aboriginal identity (https://www answer;

<operator>: you could also be interested by this study : Aboriginal Peoples: Fact Sheet for British Columbia (https://www150.statcan.gc.ca/n1/pub/89 health inside it. inform;

<user>: oh these are great! autoFeedback;

<user>: thank you so much!

<operator>: You're welcome.

# Conversation 19542

**Turns: 5**

**Messages: 18**

<user>: Hi there

<operator>: Hello, my name is Jimmy N., how may I help you? offer;

<user>: I'm looking for a table on Statistics Canada Quarterly construction price statistics catalogue 62-007 from Feb 2018 request;

<operator>: You can obtain this information at the following hyperlink : Table: 18-10-0135-02 Building construction price indexes, percentage change, quarterly (https://www150.statcan.gc.ca/t1/tbl1/en/tv.action?pid=1810013502)

<operator>: Table: 18-10-0135-01 Building construction price indexes, by type of building (https://www150.statcan.gc.ca/t1/tbl1/en/tv.action?pid=1810013501) answer;

<user>: how can I get it for monthly request;

<operator>: To view/ manipulate the variables available in a data table: â€¢ Click on "Add/Remove data" â€¢ Select at least one variable in each tab and click on â€œApplyâ€  in order to view your customized table To download the data: â€¢ Click on â€œDownloadâ€  â€¢ Select one of the three output formats then click on the hyperlink and save the table The following video may also be helpful to you:Â How to use the data tables (https://www.statcan.gc.ca/eng/sc/video/howto) .  inform; instruct;

<operator>: Unfortunately, it's a quarterly database. inform;

<operator>: The data you are requesting is not available as a standard product. However, it may be available through a custom order (a fee may apply). To obtain a free cost estimate for this service, please send us your request, clearly indicating the variables, geographic areas, time frame and data frequency needed, making sure to include your complete contact information (name of organization, address, postal code, and phone number) at the following email address:Â infostats@canada.ca (mailto:infostats@canada.ca) Â or by telephone at 1-800-263-1136. Our agents are available Monday to Friday (except holidays) from 7:30 am to 7:30 pm (Eastern Time). An agent will get in touch with you to verify the information, provide an estimate and proceed with the payment, if applicable. Please do not share any personal information through the live chat.Â Would you like to make this request? inform; instruct; infoSeekingQuestions;

<user>: not able to get monthly inform;

<operator>: The data you are requesting is not available as a standard product. However, it may be available through a custom order (a fee may apply). inform;

<user>: where can I find the release dates - I could use what ever rate that was available on feb 1 infoSeekingQuestions;

<operator>: Please hold while I find the information. timeManagement; promise;

<operator>: As of february 1st 2018, the Building construction price indexes, third quarter 2018 (https://www150.statcan.gc.ca/n1/daily-quotidien/181115/dq181115c-eng.htm) was the latest to be released on November 15th 2018 answer;

<operator>: My mistake

<operator>: That was released early 2019

<operator>: Please note that 2017 was used as the reference year on those tables. inform;

<operator>: For more information, please send an email to infostats@canada.ca (mailto:infostats@canada.ca) where an agent from the Producer Price Division will be able to assist you. instruct;

# Conversation 7703

**Turns: 2**

**Messages: 7**

<user>: Hello, I need to find out the rate for the base rent increase on January 1, 2016- January 1, 2020. As per the commercial lease, the rate is based on inflation according to the Consumer Price Index. Is there a link or a table I can refer to? inform; infoSeekingQuestions;

<operator>: Please hold timeManagement;

<operator>: You can obtain this information from our Data Table 18-10-0005-01 (https://www150.statcan.gc.ca/t1/tbl1/en/tv.action?pid=1810000501) answer;

<operator>: To view/ manipulate the variables available in a data table: • Click on "Add/Remove data" • Click on the “ + ” icon next to a checkbox to expand the list of variables (if applicable) • Select at least one variable in each tab and click on “Apply” in order to view your customized table To download the data: • Click on “Download” • Select one of the three output formats then click on the hyperlink and save the table The following video may also be helpful to you: How to use the data tables (https://www.statcan.gc.ca/eng/sc/video/howto) . inform; instruct;

<operator>: 62-557-X - Your Guide to the Consumer Price Index - ARCHIVED (calculating Percentage Changes) (http://www5.statcan.gc.ca/bsolc/olc-cel/olc-cel?lang=eng&catno=62-557-X) inform;

<user>: Ohh thank you! autoFeedback;

<operator>: You're welcome

# Conversation 5969

**Turns: 3**

**Messages: 11**

<user>: hi there

<operator>: Hello, my name is Jimmy N., how may I help you? offer;

<user>: can you please confirm when the following data table will be updated to Reflect the July 2019 popluation estiamtes? request;

<user>: https://www150.statcan.gc.ca/t1/tbl1/en/tv.action?pid=1710013501

<operator>: Please hold while I find the information. timeManagement; promise;

<operator>: I'm still doing a search, i'll get back to you shortly. timeManagement;

<operator>: The data is scheduled to be released on February 13th 2020. However the date is subject to change. answer;

<user>: thanks

<user>: ok thank you autoFeedback;

<operator>: You're welcome!

<operator>: We are currently evaluating our customer service. Your input would be much appreciated: www.statcan.gc.ca/survey/SIS (http://www.statcan.gc.ca/survey/SIS) Thank you! request;

# Conversation 6650

**Turns: 12**

**Messages: 34**

<user>: Hello. I can see that in 2015 there was a CCHS nutrition focus survey completed. Can you point me in the direction of any data tables or information from that survey. It says that data was rele ased in 2017 request;

<operator>: Hello, my name is Kevin, let me look into this for you. timeManagement; promise;

<user>: thank you

<operator>: Here are all the created tables from the CCHS - Nutrition:Canadian Community Health Survey - Nutrition - Data Tables (https://www150.statcan.gc.ca/n1/en/surveys/5049) answer;

<user>: yes i found that, but i cannot find any information released from the 2015 nutrition focus. inform;

<user>: https://www.canada.ca/en/health-canada/services/food-nutrition/foodnutrition-surveillance/health-nutrition-surveys/canadian-community-health-survey-cchs/2015-canadiancommunity-health-survey-nutrition-food-nutrition-surveillance.html

<user>: it is referenced there and states that data was released in 2017 inform;

<operator>: Please hold. timeManagement;

<user>: thank you

<operator>: The survey was indeed done in 2015 and most of the tables in the sent link were released in 2017.

<operator>: The CCHS nutrition was not conducted after 2015 therefore all the tables are from that survey answer;

<user>: i cannot find anything related to that data. can you point me in the right direction. Just looking for any data tables or results inform; request;

<user>: i cannot find any tables that reference the 2015

<operator>: Were you able to access the link we sent you? 16/01/2020 2/2 clarificationQuestion;

<operator>: On the "Data" tab, you will find the requested tables instruct;

<operator>: Canadian Community Health Survey - Nutrition - Data Tables (https://www150.statcan.gc.ca/n1/en/surveys/5049) inform;

<user>: yes - this is the one i was interested in but it says it is for 2004 only 22. Household food insecurity Table: 13-10-0472-01 (formerly: CANSIM 105-2004) Geography: Canada, Province or territory Frequency: Occasional Description:Number and percentage of persons based on the level of household food insecurity, by age group and sex, for 2004 only. answer;

<operator>: We would have this table from the Annual CCHS:Household food insecurity, by age group and food insecurity status (https://www150.statcan.gc.ca/t1/tbl1/en/tv.action?pid=1310046301)

<operator>: Released in 2014, but nothing more recent. inform;

<user>: yes, i am wondering why it was included as part of the nutrition focus in 2015 but there is no data available infoSeekingQuestions;

<operator>: My apologies, we also have this one from this year: Household food security by living arrangement (https://www150.statcan.gc.ca/t1/tbl1/en/tv.action?pid=1310038501) answer;

<user>: looking for what was included as part of the 2015 nutrition focus request;

<operator>: It appears they changed the table name from Food Insecurity in 2004 to Food Security answer;

<user>: it still doesn't provide the data from 2015 inform;

<operator>: Please hold. timeManagement;

<operator>: Statistics Canada released the 2015 CCHS Nutrition data on June 20th, 2017, making it available to researchers through the Data Research Centres and to its share partners, Health Canada and Public Health Agency of Canada. answer;

<operator>: This is the reason why the Food Security table is not available on our website.

<operator>: The only tables available on our website regarding the 2015 CCHS - Nutrition are the percentage of total energy intake from fats, carbohydrates and protein, total energy,

nutritional supplement consumption, nutrients from supplements, body mass index as well as children's physical activity and screen time inform;

<user>: okay. so this information could be available but is not available on the website. autoFeedback;

<user>: thank you

<operator>: That is correct. answer;

<user>: thank you

<operator>: You're welcome!

<user>: can you tell me one more thing? request;

# Conversation 22159

**Turns: 8**

**Messages: 19**

<user>: hi

<operator>: hello

<operator>: how may i help you today? offer;

<user>: screenshot.lzsc (https://www.statcan.gc.ca/livechat/getfile.php?file=screenshot.lzsc&id=2e1ea895e5d3855b421a8909c06f6449)

<user>: What does these number mean? infoSeekingQuestions;

<operator>: sorry i can't see your screenshot inform;

<user>: Are these $ value? clarificationQuestion;

<operator>: can you send me the link? infoSeekingQuestions;

<user>: https://www150.statcan.gc.ca/t1/tbl1/en/cv.action?pid=1810000501#timeframe answer;

<operator>: those are not in dollar inform;

<user>: in thousand??

<operator>: https://www.statcan.gc.ca/eng/subjects-start/prices_and_price_indexes/consumer_price_indexes/faq

(https://www.statcan.gc.ca/eng/subjects-start/prices_and_price_indexes/consumer_price_indexes/faq)

<user>: per year?? correct? infoSeekingQuestions;

<operator>: there are not interpreted in $ values on the table otherwise it would be indicated in the title answer;

<operator>: please refer to the link i sent you regarding the CPI request;

<user>: if they are not $value then what r they? clarificationQuestion;

<operator>: it is just an index value inform;

<operator>: https://www.statcan.gc.ca/eng/subjects-start/prices_and_price_indexes/consumer_price_indexes/faq (https://www.statcan.gc.ca/eng/subjects-start/prices_and_price_indexes/consumer_price_indexes/faq)

<user>: thx bye

# Conversation 20791

**Turns: 1**

**Messages: 4**

<user>: I am looking for the new table that replaced CANSIM 326-0020 - what is the new table name? request;

<operator>: Please hold timeManagement;

<operator>: This is the data table 18-10-0004-13 (https://www150.statcan.gc.ca/t1/tbl1/en/tv.action?pid=1810000413&request_locale=en) answer;

<operator>: To view/ manipulate the variables available in a data table: â€¢ Click on "Add/Remove data" â€¢ Click on the â€œ + â€  icon next to a checkbox to expand the list of variables (if applicable) â€¢ Select at least one variable in each tab and click on â€œApplyâ€ in order to view your customized table To download the data: â€¢ Click on â€œDownloadâ€ â€¢ Select one of the three output formats then click on the hyperlink and save the table The following video may also be helpful to you:Â How to use the data tables (https://www.statcan.gc.ca/eng/sc/video/howto) .  inform; instruct;
